# Supplementary material for: Dispersion for Data-Driven Algorithm Design, Online Learning, and Private Optimization
Source: arXiv:1711.03091 source file (2018-10-22)
Supplement: Supplementary file 1 [file lower_bounds_appendix.tex]

First, we fix some notation that we will need to prove this section's main theorem. We assume that $u(x, \rho)$ is the total weight of the independent set returned by the algorithm parameterized by $\rho$ given the input instance $x$. For a sample $\sample \subseteq \Pi$ of MWIS problem instances, let $I_{\sample}$ be the set of empirically optimal parameters.

\begin{lem}[Lemma 4.1 from \citep{Gupta16:PAC}]\label{lem:Gupta_WC}
For any constants $0 < r < s< 1$ and any $t \geq 2$, there exists a MWIS instance $x$ on $t^3 + 2t^2 + t - 2$ vertices such that $u(x, \rho) = 1$ when $\rho \in (r,s)$ and $u(x, \rho) \leq \frac{t^r(t^2 - 2) + t^{-s}(t^2 + t + 1)}{t^3 - 1}$ when $\rho \in [0,1] \setminus (r,s)$.
\end{lem}

We will also use the following theorem from De's work, revised for our setting.
\begin{theorem}[Theorem 1 from \citep{De12:Lower}]\label{thm:de}
Assume $\sample_1, \dots, \sample_{2^s} \in \Pi^N$ are samples such that for $i \not= j$, $\left|\sample_i \Delta \sample_j\right| \leq \Delta$ and $\min_{\rho \in I_{\sample_i}, \rho' \in I_{\sample_j}}|\rho-\rho'| \geq \eta$. For any $\epsilon >0$, if $\Delta \leq (s-1)/\epsilon$, then for any $\epsilon$-differentially configuration algorithm $\alg$ there exists a sample $\sample_i$ such that \[\Pr_{\rho' \sim \alg(\sample_i)} \left[ \min_{\rho \in I_{\sample}} |\rho' - \rho| > \frac{\eta}{2}\right] \geq \frac{1}{2}.\]
\end{theorem}

\begin{restatable}{theorem}{worstCase}\label{thm:main_worst_case}
 Let $n \geq 46$, $\epsilon >0$, $N > \frac{1}{2\epsilon}$, and let $\alg$ be any $\epsilon$-differentially private algorithm. There exists a distribution $\mathcal{D}$ over MWIS instances with $n$ nodes such that with probability at least $1/2$ over the draw of $\sample \sim \mathcal{D}^N$ and $\rho' \sim \alg(\sample)$, $\E_{x \sim \dist}[u(x, \rho')] < \max_{\rho}\E_{x \sim \dist}[u(x, \rho)] - 1/5.$
\end{restatable}

\begin{proof}
Let $t$ be any integer greater than 3 such that $t^3 + 2t^2 + t - 2 \leq n$ and let $x_1, x_2, \dots, x_k$ be $k:= 2^{2N \epsilon + 1}$ MWIS instances on $t^3 + 2t^2 + t - 2$ nodes guaranteed to exist by Lemma~\ref{lem:Gupta_WC}, such that $x_i$ is defined by the values $r_i > 0.49$ and $s_i < 0.51$ and such that for $i \not= j$, $[r_i, s_i] \cap [r_j, s_j] = \emptyset$. Let $\sample_1, \dots, \sample_k$ be $k$ samples such that $\sample_i$ consists of $N$ copies of instance $x_i$. Notice that $|\sample_i \Delta \sample_j| = 2N$ for all $i \not= j$, so we may apply Theorem~\ref{thm:de} with $\Delta = 2N$ and $s = 2N \epsilon + 1$. In particular, this means that for some $i^*$, $\Pr\left[\min_{\rho \in I_{\sample_{i^*}}} |\rho' - \rho| > 0\right] \geq \frac{1}{2}$.

Next, let $\mathcal{D}$ be the distribution such that with probability 1 over the draw of a sample $x \sim \dist$, $x = x_{i^*}$. We know that if $\rho \in I_{\sample_{i^*}}$, then $u\left(x_{i^*}, \rho\right) = 1$ and otherwise, \[u\left(x_{i^*}, \rho\right) \leq \frac{t^r(t^2 - 2) + t^{-s}(t^2 + t + 1)}{t^3 - 1} \leq \frac{t^{0.51}(t^2 - 2) + t^{-0.49}(t^2 + t + 1)}{t^3 - 1}\leq 0.8\] for $t\geq 3$. Therefore, with probability 1 over the draw of the sample $\sample \sim \dist^N$ and probability at least $1/2$ over the draw of the output $\rho' \sim \alg(\sample)$, we have that $\E_{x \sim \dist}\left[u\left(x, \rho'\right)\right] \leq 0.8 < 1 = \max_{\rho}\left\{\E_{x \sim \dist}\left[u\left(x, \rho\right)\right]\right\}$, so the theorem statement holds.
\end{proof}
