# Supplementary material for: Dispersion for Data-Driven Algorithm Design, Online Learning, and Private Optimization
Source: arXiv:1711.03091 source file (2018-10-22)
Supplement: Supplementary file 2 [file figures_appendix.tex]

\begin{figure}
  \centering
  \includegraphics[width=0.3\textwidth]{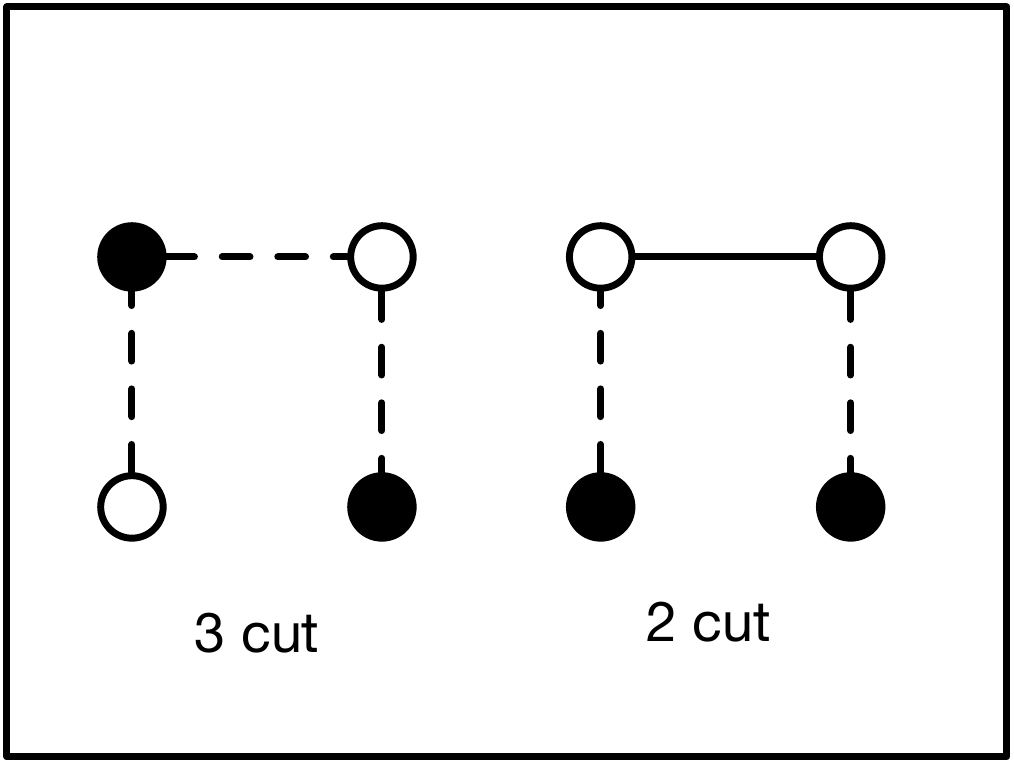}
  \caption{Examples of two cuts for the max-cut problem. The left example cuts
  3 edges and is optimal, while the right example only cuts two. In the max-cut
  problem, the goal is to color the nodes black and white to maximize the number
  of edges from black to white nodes.}
  \label{fig:maxcut}
\end{figure}

\begin{figure}
  \begin{subfigure}[t]{0.45\linewidth}
    \centering
    \includegraphics[width=0.7\textwidth]{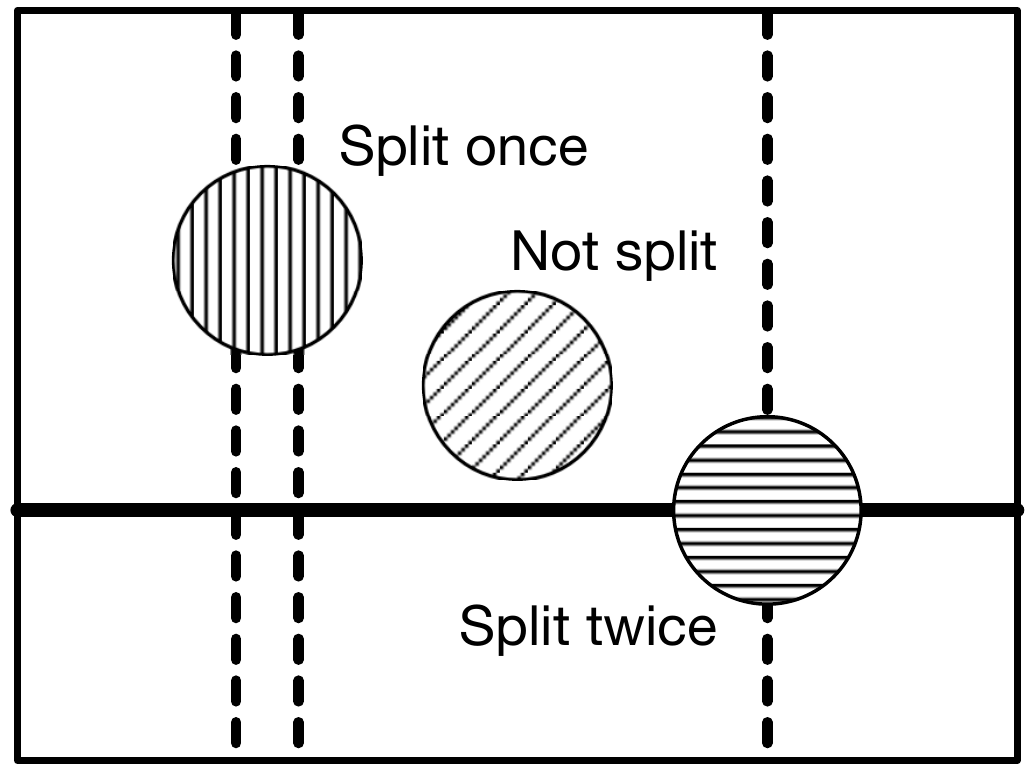}
    \caption{The dashed and solid lines correspond to two partitionings of the
    rectangle. Each of the displayed balls is either not split, split by one
    partition, or split by both.}
    \label{fig:splitting}
  \end{subfigure}
  \hfill
  \begin{subfigure}[t]{0.45\linewidth}
    \centering
    \includegraphics[width=0.7\textwidth]{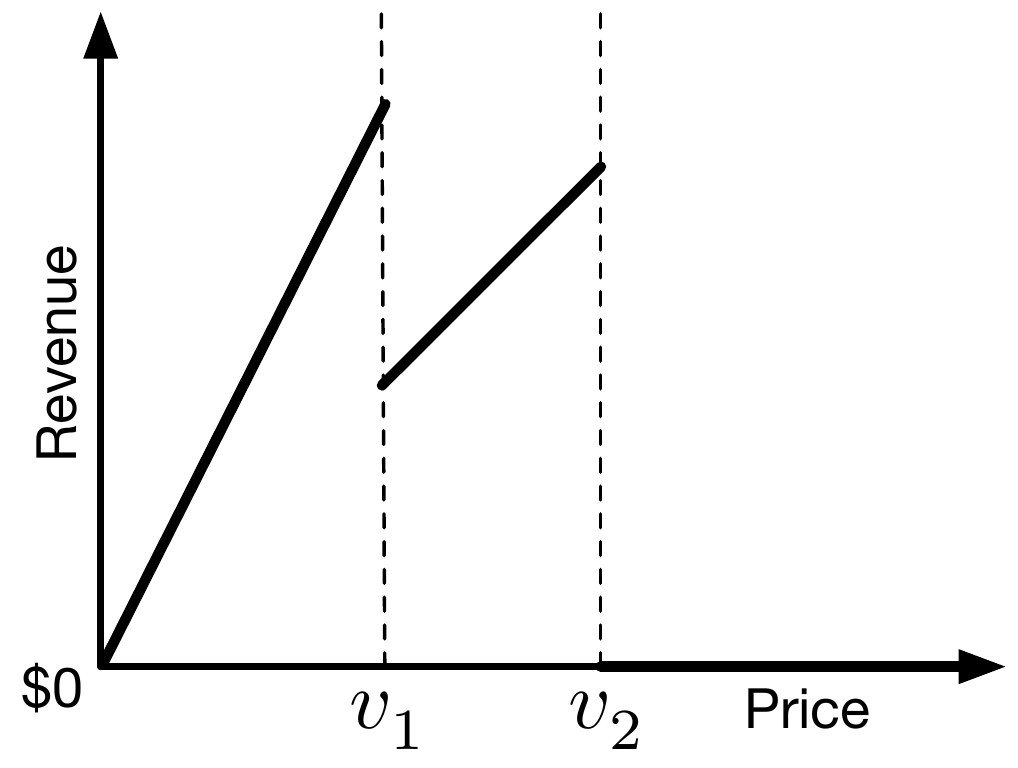}
    \caption{The total revenue generated when offering a digital good at a given
    price to two sample buyers with values $v_1$ and $v_2$. This function has
    discontinuities at each buyer valuation.}
    \label{fig:pricing}
  \end{subfigure}
  \caption{}
\end{figure}
